# Supplementary material for: The study of r-process nucleosynthesis in binary neutron star mergers: Nucleonic weak interactions and nuclear uncertainties
Source: arXiv:2303.06366 source file (2023-03-11)
Supplement: Supplementary file 1 [file appendixA.tex]

\chapter{The First Appendix}
\label{sec:first-app}
\kant[20-21] % Dummy text
\section{First Section}
\kant[22]    % Dummy text
\section{Second Section}
\kant[23-24] % Dummy text
