# Supplementary material for: The study of r-process nucleosynthesis in binary neutron star mergers: Nucleonic weak interactions and nuclear uncertainties
Source: arXiv:2303.06366 source file (2023-03-11)
Supplement: Supplementary file 2 [file appendixB.tex]

\chapter{Source Code}
\label{sec:source}
\section{Implementation}

Example code \texttt{read\_qvals.f90}
\lstinputlisting[language = {[95]{Fortran}}]{read_qvals.f90}
